# Supplementary material for: Determining Surface Phase Diagrams Including Anharmonic Effects
Source: arXiv:1908.11118 ancillary file (2019-08-29)
Supplement: Supplementary file 1 [file Zhou_ReplicaExchangeGrandCanonical_2019_SI.pdf]

**Supplementary Information to**
**Determining Surface Phase Diagrams including Anharmonic Effects**

Yuanyuan Zhou, Matthias Scheffler, and Luca M. Ghiringhelli
*Fritz-Haber-Institut der Max-Planck-Gesellschaft, Berlin-Dahlem, Germany*

27 August 2019

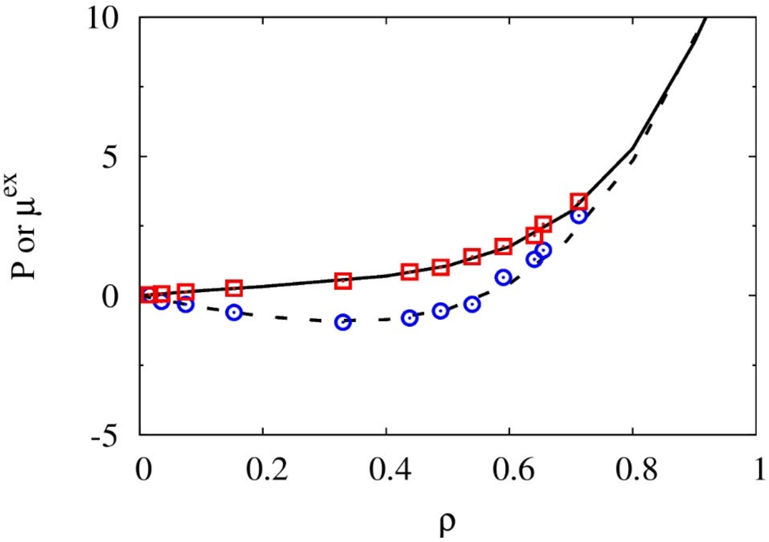


FIG. S1. Equation of state of the Lennard-Jones fluid; isotherm at T = 2.0. The solid line is the equation of state of Johnson et al. [Molecular Physics 78, 591 (1993)] and the squares are the results from our grand-canonical simulations. The dotted line is the excess chemical potential as calculated from the equation of state of Johnson et al [Molecular Physics 78, 591 (1993)] and the circles are the results of the simulations. All variables are in reduced units. The translation of reduced units to real units for Lennard-Jones argon are the same in Ref [D. Frenkel and B. Smit, Understanding molecular simulation: From algorithms to applications (Elsevier, 2002).]

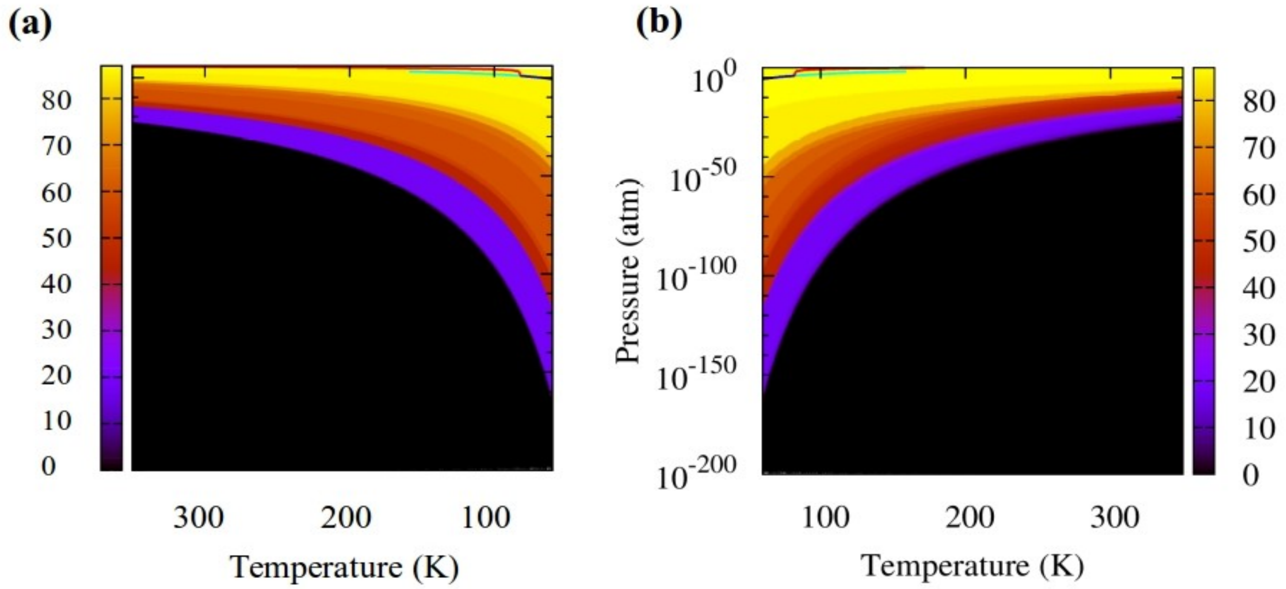


FIG. S2. Phase diagrams of a LJ gas-phase (particles B) in contact with a frozen fcc(111) LJ frozen surface calculated by and aiAT (a) and MBAR (b) at low temperatures conditions ranging from 60 to 350 K.

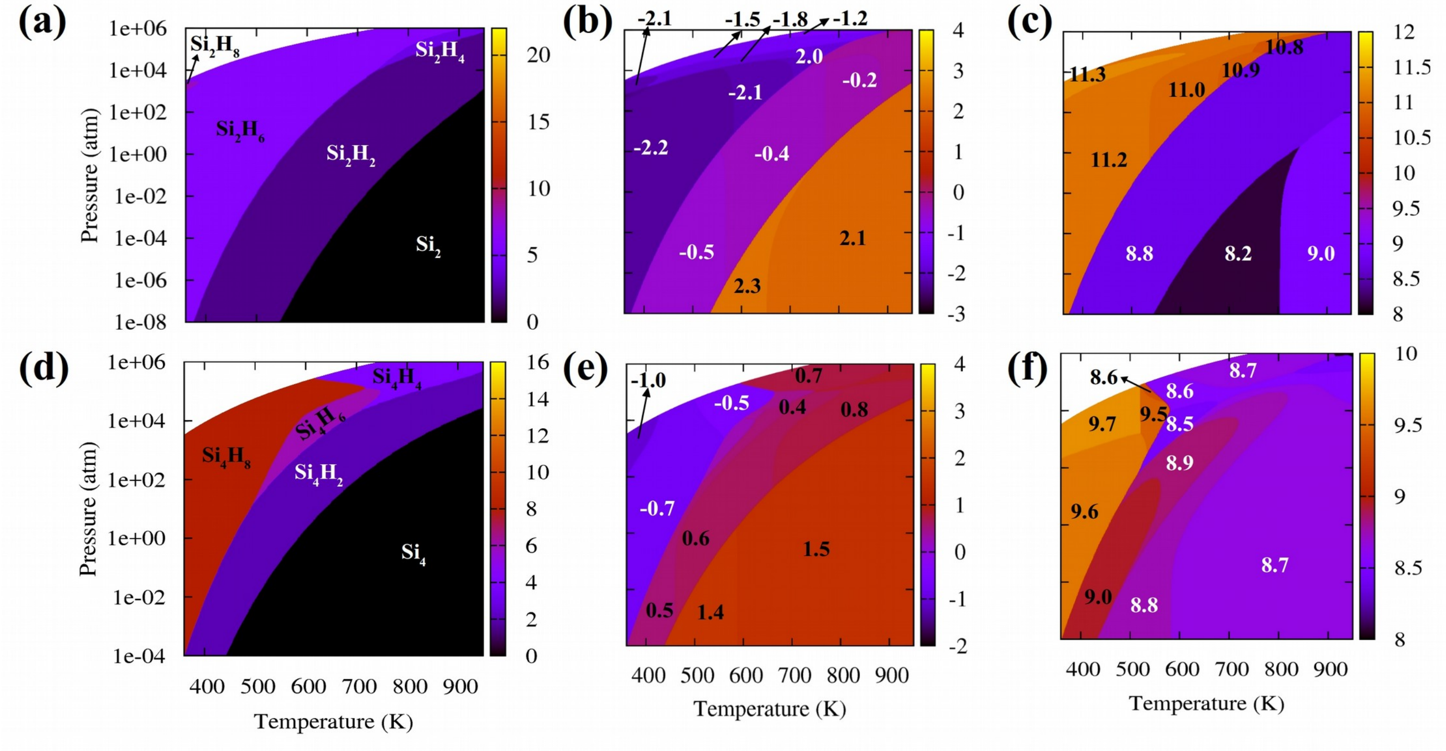


Fig. S3 Phase diagrams of chemisorbed $Si_2H_N$ (a), vertical electronic affinity (VEA) (b) and vertical ionization potential (VIP) (c) of $Si_2H_N$ at reactive gas phase, respectively. Phase diagrams of chemisorbed $Si_4H_N$ (a), vertical electronic affinity (VEA) (b) and vertical ionization potential (VIP) (c) of $Si_4H_N$ at reactive gas phase, respectively. The scale of panels (a) and (d) is the number of chemically adsorbed H atoms. VEA and VIP in panels (b), (c), (e) and (f) are in eV.

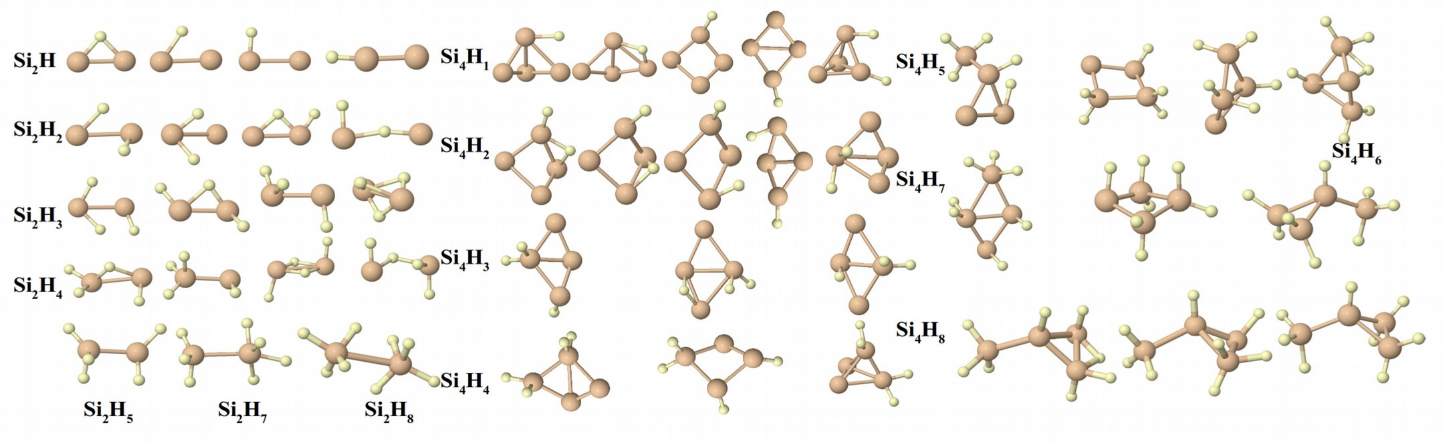


FIG. S4. Structures of isomers of each $Si_{\{2,4\}}$ with $H_N$ size, respectively.

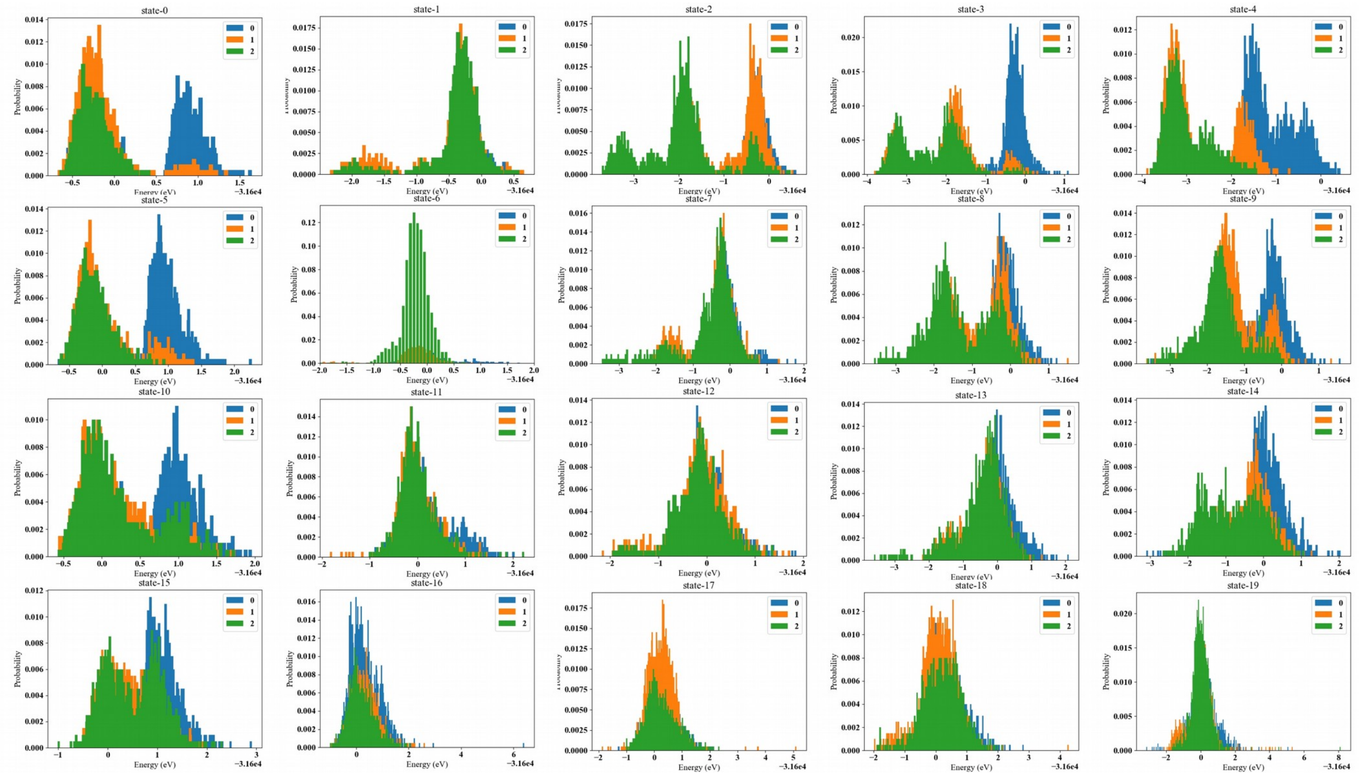


FIG. S5. Distribution of *adsorption energy* ($E_{Si_4H_N}$-$N/2E_{H_2}$) of each thermodynamical state in the REGCMD simulation for $Si_4$. Each trajectory is divided into three same interval (2000 REGCMD steps). The distribution is calculated at every interval for each trajectory. The blue, orange and green bars indicate the energy distribution of first, second and third interval of each trajectory, respectively.

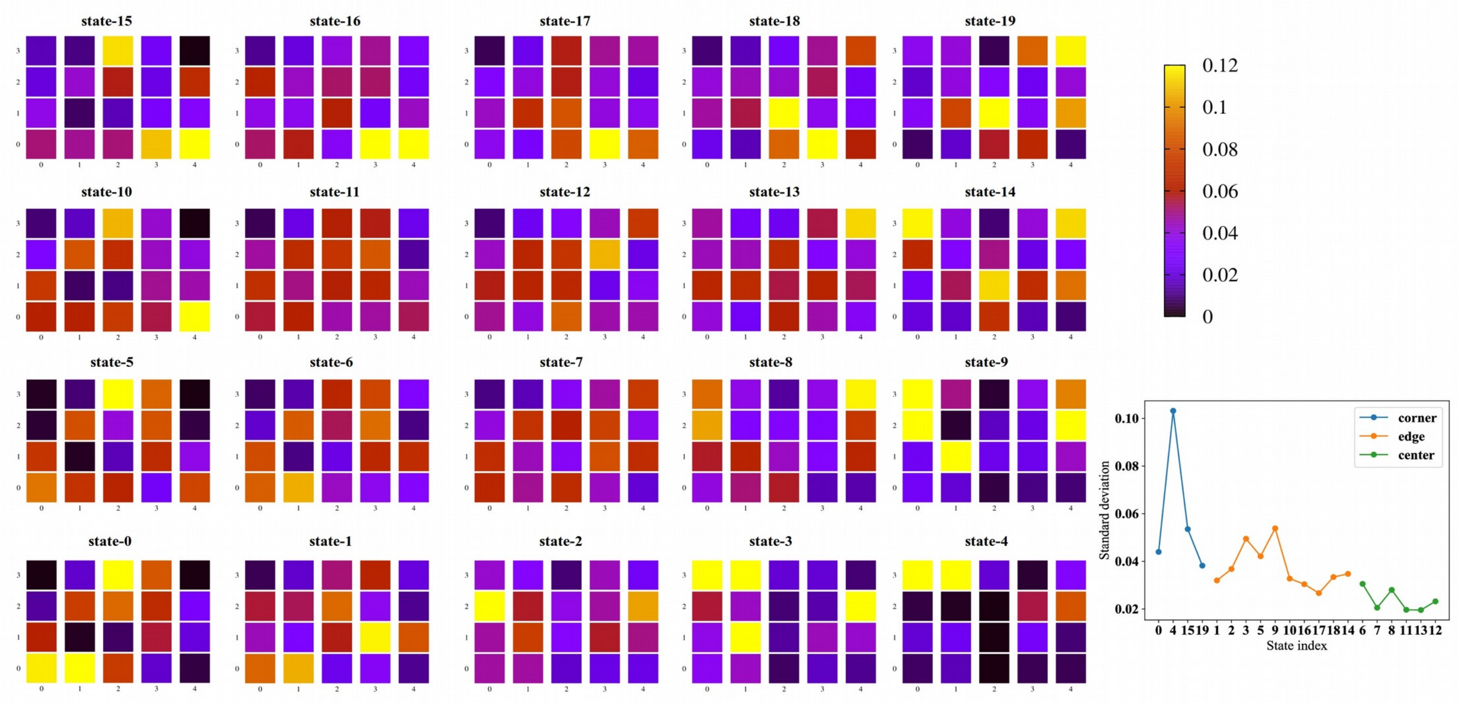


FIG. S6. The diffusion probability of each thermodynamical state in each configuration (replica) in the REGCMD simulation for $Si_4$; Inset on the bottom right: the standard deviation of each state.
